# Supplementary material for: Second Dome of Superconductivity in YBa$_2$Cu$_3$O$_7$ at High Pressure
Source: arXiv:2305.05715 ancillary file (2024-04-18)
Supplement: Supplementary file 1 [file supplemental_material.pdf]

# Supplemental material: Candidate for Second Dome Superconductivity in $YBa_2Cu_3O_7$ at High Pressures

Johannes Nokelainen[1,2,3,*], Matthew E. Matzelle[1], Christopher Lane[4], Nabil Atlam[1], Ruiqi Zhang[5], Robert S. Markiewicz[1], Bernardo Barbiellini[3,1], Jianwei Sun[5], and Arun Bansil[1,†]

[1]*Department of Physics, Northeastern University, Boston, Massachusetts 02115, USA*
[2]*Department of Physics and Astrophysics, Howard University, Washington, D.C 20059, USA*
[3]*Department of Physics, School of Engineering Science, LUT University, FI-53850 Lappeenranta, Finland*
[4]*Theoretical Division, Los Alamos National Laboratory, Los Alamos, New Mexico 87545, USA*
[5]*Department of Physics and Engineering Physics, Tulane University, Louisiana 70118 New Orleans, USA*
[*]j.nokelainen@northeastern.edu
[†]ar.bansil@northeastern.edu

## S1 Computational details

The DFT simulations were carried out using the Vienna *ab initio* simulation package (VASP) [29–31]. The exchange-correlation energy was treated within the SCAN meta-GGA scheme [32]. The choice of the SCAN functional is discussed in detail in the Sec. S1.3. In the relaxation and band structure calculations we employed a Gaussian smearing with a width of 0.05 eV. The tetrahedron method with Blöchl corrections was used for obtaining accurate DOS and energy values. When analyzing the energetics of various magnetic states that are presented in the main text Fig. 2 (b), we used values of enthalpy $H$, which is the appropriate thermodynamic quantity under pressure, given in the VASP output. A total energy tolerance of $10^{-5}$ eV was used in both relaxation and DOS calculations.

### S1.1 Structures and their relaxation

We employed a 26-atom $\sqrt{2} \times \sqrt{2}$ supercell for the calculations of pressure evolution of the C-AFM, G-AFM and NM phases and the AFM phase electronic structure calculations, see the main text Figs. 1 (d), 2, 3 (a), 3 (b) and 4. We used the $\sqrt{2} \times \sqrt{2}$ supercell also for the $YBCO_6$ reference structure (24 atoms) in the hole-content analysis, see Fig. 2 (a) and Sec. S3. For the stripe phase calculations that are discussed later in Sec. S4, we used 78-atom $3 \times 2$ and $2 \times 3$ supercells. We used the 13-atom primitive cell for the electronic structure of the 100 GPa NM state shown in Fig. 3 (c). We performed the phonon calculations, which are discussed in Sec. S6, in a $2 \times 2 \times 2$ supercell. Note that the structure shown in Fig. 1 (a) depicts a $2 \times 2$ supercell for visualization purposes, although it was not used in our calculations.

Table S1: Used real and momentum-space grid densities.

| Structure | Real-space grid | $k$-space grid |
|---|---|---|
| $YBCO_7$, primitive cell | $120 \times 120 \times 360$ | $16 \times 16 \times 4$ |
| $YBCO_7$, $\sqrt{2} \times \sqrt{2}$ supercell | $160 \times 160 \times 360$ | $12 \times 12 \times 4$ |
| $YBCO_7$, $2 \times 3$ supercell | $240 \times 360 \times 360$ | $8 \times 6 \times 4$ |
| $YBCO_7$, $3 \times 2$ supercell | $360 \times 240 \times 360$ | $6 \times 8 \times 4$ |
| $YBCO_7$, $2 \times 2 \times 2$ supercell | $240 \times 240 \times 720$ | $8 \times 8 \times 2$ |
| $YBCO_6$, $\sqrt{2} \times \sqrt{2}$ supercell | $160 \times 160 \times 368$ | $12 \times 12 \times 4$ |

When computing the relative enthalpies ($H_{\mathrm{AFM}} - H_{\mathrm{NM}}$), we used the NM supercell equal in size to the AFM supercell rather than scaling up the NM primitive cell energy. This was done in order to eliminate inaccuracies that such scaling could have due to subtle technical reasons and thus ensure compatibility between these calculations.

We employed a dense real-space grid in order to improve the accuracy of the Bader analysis, see Sec. S3, and also a dense $k$-space grid in order to stabilize the high-pressure magnetic moments, see Sec. S1.4. These grids correspond to real-space density of about 30 grid points per ångström and a $k$-point density of about $0.015 \times \frac{2\pi}{\text{Å}}$, except for the $c$-direction, where we used a slightly coarser $k$-space grid density of about $0.02 \times \frac{2\pi}{\text{Å}}$. These densities are for ambient pressure. When the structures become compressed under pressure, the real-space ($k$-space) grid densities increase (decrease) since the number of grid points used was kept constant. We have summarized the number of grid points used for each structure in Table S1.

All structures were fully relaxed until an atomic force tolerance of 0.02 eV/Å was reached. No constraints on the unit cell shape or volume nor the atomic positions were placed with the exception of the hydrostatic pressure, which we took into account by subtracting the pressure value from the diagonal elements of the stress tensor through the `PSTRESS` flag, leading the system to automatically compress to the pressurized structure. We applied the pressure adiabatically, always starting from the structure obtained from the previous step and then increasing the pressure by a small value for the new relaxation.

## S1.2 Oxygen potentials and plane-wave energy cutoff

Our DFT simulations were carried out using the projector-augmented-wave (PAW) method [29,30]. For VASP, there are both "soft" and "hard" oxygen PAW potentials available, with large and small PAW sphere radii of 0.820 Å and 0.595 Å, respectively. We used the hard oxygen potentials since for the soft potentials the O and Cu PAW spheres overlap at high pressures (Cu PAW sphere has a radius of 1.218 Å), which led to errors in our tests. For the soft oxygen potential there actually is a slight Cu–O overlap of 0.08 Å already at ambient pressure, but such small overlaps did not lead to problems in

our tests since we obtained identical low-pressure results with the soft and hard potentials. Even with the hard potential small overlaps were encountered at the highest pressures, suggesting that increasing pressure much beyond the studied 170 GPa range may lead to decreased accuracy.

The usage of the hard potentials requires a high energy cutoff for the plane-wave basis in the expansion of the Kohn-Sham orbitals. We used particularly high value of 950 eV for reasons discussed in Sec. S1.4.

## S1.3 Choice of the SCAN exchange-correlation functional

Our decision to use the SCAN functional [32] is based on results in the literature, our previous experience, and the benchmarking tests that we conducted on $YBCO_7$.

In the earlier studies [33–41] SCAN has been shown to provide good description of materials for which the dominant physics involves strong correlations, *pd*-hybridization and charge transfer. We emphasize that the functional benchmarking by Pokharel *et al.* [38] focuses on the cuprates. Ref. 38 shows that the traditional local density approximation (LDA) and generalized gradient approximation (GGA) functionals have difficulties in describing the magnetic properties of the cuprates and require an external Hubbard $U$ parameter. The value of $U$ needed to correctly capture physical properties is different for various properties. In contrast, SCAN has been shown to reasonably capture many salient features of the electronic structures of the cuprates, including stabilization of the magnetic states without any external parameters.

We have conducted functional benchmarking tests on $YBCO_7$ by comparing GGA, GGA + $U$ and SCAN based results. We used the GGA parametrization of Perdew, Burke and Ernzerhof (PBE) [77]. As the first step we investigated the effects of correlation and choice of functional on the high-pressure NM state. The earlier YBCO studies conducted with GGA + $U$ have considerable variation for the $U$ parameter value, going as high as 9 eV [78], which we used in this first test. Figure S1 presents the resulting electronic structures and they have little variation despite the large $U$ value used. Only slight energy shifts are visible. This is in line with our previous results on the cuprates. Suppressing magnetism (`ISPIN = 1`) and thus also the correlation effects was found to yield very similar NM electronic structures between the GGA and SCAN, independent of the exact compound or pressure. However, the differences in the structural parameters can still be considerable between the GGA and SCAN. In the case of 100 GPa $YBCO_7$, we obtained only small differences in the lattice constants between the GGA and SCAN, but this makes sense since one of the main structural effects of SCAN in materials such as $YBCO_7$ is to improve the description of the weak interactions over the van der Waals gap, which become negligible at high pressures. Since the SCAN structural parameters were in excellent agreement with experiment below 13 GPa, as discussed in the main text, these SCAN and PBE structural parameters at 100 GPa are also likely to be robust. However, PBE + $U$ = 9 eV led to considerable ($\sim 1\,\%$) shrinkage of the $a$ and $b$ parameters.

As a second test we investigated the ambient-pressure C-AFM state with PBE + $U$ for various $U$ values. Here, we found that Cu magnetic moments increase with increasing $U$. $U = 1.5$ eV was required to

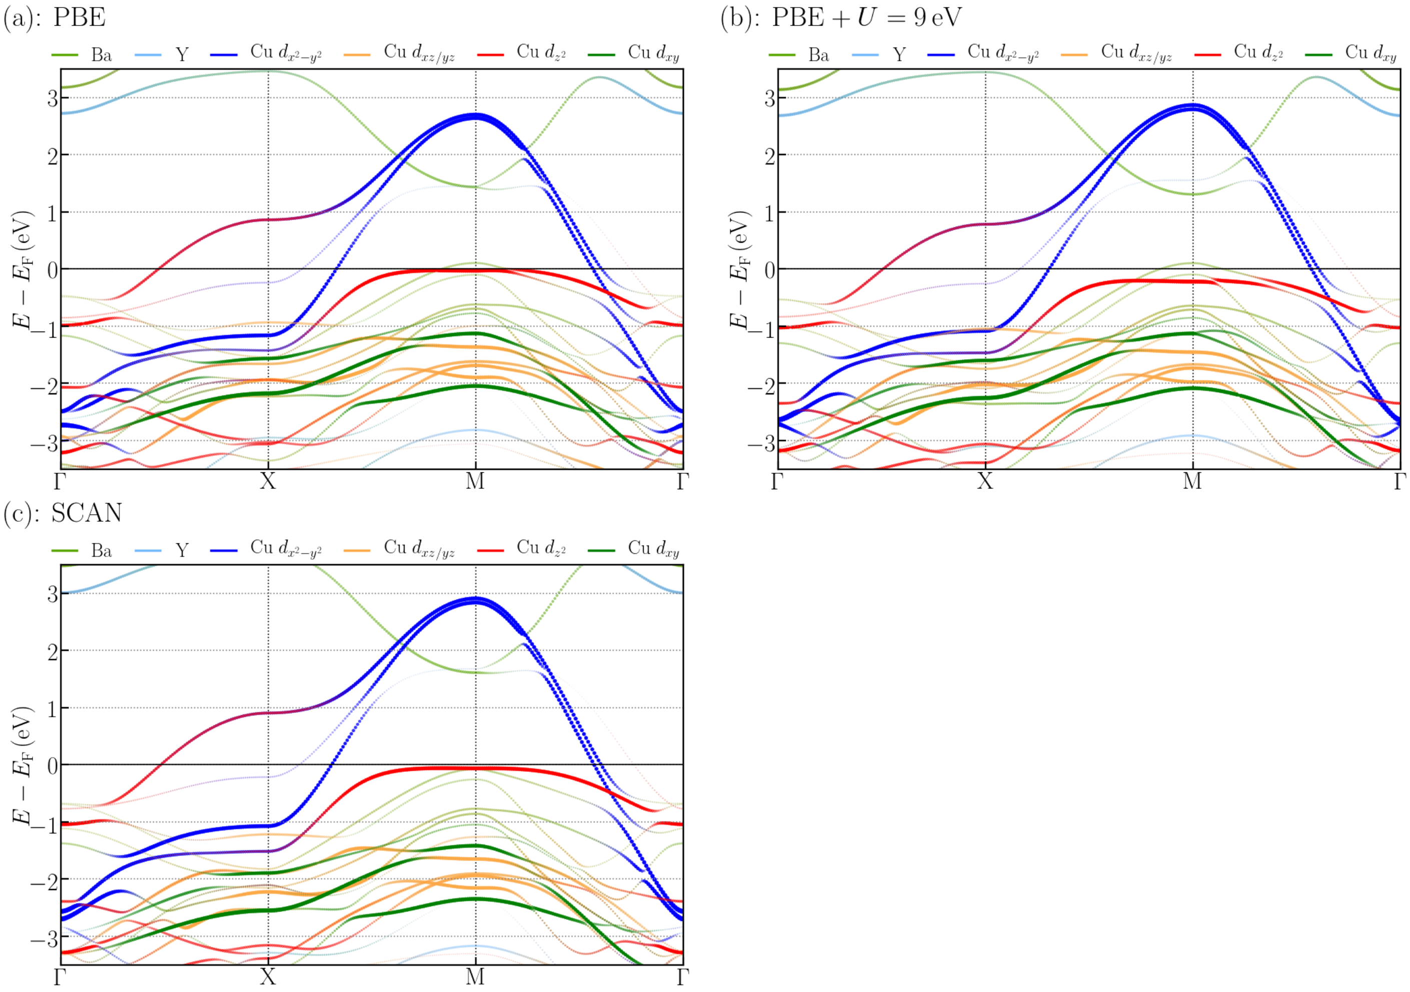


Figure S1: The 100 GPa NM band structure calculated with (a): PBE; (b): PBE + $U$ with $U$ value of 9 eV applied on the Cu atoms; (c): SCAN functional. In each case the system has also been relaxed. Differences seem to be largest for the $d_{z^2}$-band near the $M$-point.

stabilize the C-AFM state, with magnetic moment $M = 0.215\,\mu_B$. At $U = 3.5$ eV, we obtained a result roughly equal to that of SCAN, $M = 0.465\,\mu_B$. For $U = 6$ eV and 9 eV we obtained $M = 0.583\,\mu_B$ and $0.714\,\mu_B$, respectively. These values are too large since $M = 0.5\,\mu_B$ is the expected value for the half-filled case without doping ($YBCO_6$), therefore, a smaller value is expected for the doped compound $YBCO_7$. Judging by the magnetic moments, a reasonable choice of $U$ would probably be about 3–4 eV. The C-AFM state band structure is also similar for PBE + $U$ = 3.5 eV and SCAN.

With PBE+U we found another magnetic state with C-AFM-type coupling of the $Cu_{pl}$ magnetic moments but also with small ferromagnetic moments localized on the apical and chain oxygen ions that lead to a net magnetization of about $0.5\,\mu_B$ in the $\sqrt{2} \times \sqrt{2}$ supercell. This magnetized C-AFM state was found to be nearly degenerate with the C-AFM state and had lower energy than the C-AFM state for $U \geq 3.5$ eV. Such global magnetization is one possible mechanism for killing superconductivity and we have previously found similar onset of global magnetization with SCAN calculations in BSCCO, but

in a context where superconductivity is expected to vanish due to overdoping [35]. However, $YBCO_7$ is only slightly overdoped, so the emergence of such a state is not expected. It could be that PBE $+ U$ is not properly capturing the charge transfer effects in YBCO.

## S1.4 Stabilizing the magnetic states at high pressures

We had to pay special attention to the computational details to obtain robust results on the magnetic states and preserve the magnetic moments under high pressures. Firstly, it was necessary to use especially high $k$-space grid density of $0.015 \times \frac{2\pi}{\text{Å}}$ and a high plane-wave energy cutoff of 950 eV, as discussed in Secs. S1.1 and S1.2. These values were chosen to make sure that the highest-pressure G-AFM and C-AFM states retained their magnetic moments.

Secondly, at high pressures only the tetrahedron method with Blöchl corrections for the Kohn-Sham orbital partial occupancies was able to properly stabilize the magnetic moments; at very high pressures the Gaussian smearing failed to find the magnetic moments. Note that the tetrahedron method is the most accurate smearing method since it interpolates the partial occupancies between the $k$-grid points. Therefore, in the structural relaxation calculations (with Gaussian smearing), magnetic moments differed from those in the final enthalpy and electronic structure calculations (with tetrahedron method smearing), but switching on the tetrahedron method did not induce significant forces on the Cu atoms, indicating that the Gaussian-relaxed structures were suitable for the final DOS and total energy calculations with the magnetic moments.

Thirdly, several ionic steps were needed to converge the magnetic moments. Restarting a calculation always yielded smaller Cu magnetic moments in the first ionic steps than in the original calculation, even though the calculation fully converged. After several steps the magnetic moment finally converged to the original value. This technical issue might be due to the fact that SCAN and other meta-GGA functionals do not load the electronic state exactly when a calculation is restarted since the kinetic-energy-related quantities are not saved for a new calculation. Furthermore, since different magnetic states are almost degenerate at high pressures, it was possible to converge into several different magnetic states at different ionic steps. Therefore, to obtain high-quality high-pressure DOS, band structure and Fermi surfaces, we used the setting `IBRION=-1` to perform several ionic steps while keeping the structure constant.

## S1.5 Fermi surface (spectral function at the Fermi energy) and band structure calculations

We unfolded [55] the band structures and spectral functions at the Fermi energy (Fig. 3) from the supercells into the primitive cell Brillouin zone using the PyProcar [56] code. In practice, an unfolding weight was assigned for each energy eigenvalue which was then taken into account as an alpha value in the plotting together with the orbital projection weights.

We calculated the Fermi surfaces (spectral functions at the Fermi energy) for a given $k$-point by dividing each energy eigenvalue into orbital and atomic contributions and then assigned a Gaussian smearing of 23 meV to them and summed together the values of these distribution functions at the Fermi energy. The smearing value was chosen small enough to provide crisp features but large enough to display the faint $d_{z^2}$ contribution close to $M$ for the 100 GPa NM case in Fig. 3 (c). We calculated the spectral functions with a resolution of $51 \times 51$ $k$-points.

The band structures and spectral functions were calculated self-consistently since SCAN and other meta-GGA functionals do not allow non-self-consistent calculations due to the quantities related to the kinetic energy density not being reloaded from the previous calculation. Therefore, the band structure and spectral function calculations were otherwise normal calculations of the electronic state of the system, but with the band structure $k$-path and the spectral function grid $k$-points being appended to the $k$-point list with zero weights.

The 100 GPa C-AFM band structure and spectral function presented in Fig. 3 (b) were calculated with the tetrahedron smearing in order to preserve the high-magnetic-moment electronic state at high pressures (see Sec. S1.4). Note that the combination of tetrahedron smearing and manually defined $k$-point list is possible only in VASP version 5, which contains a slightly bugged version of SCAN that has been fixed for VASP version 6. For this purpose, we used our own patch for VASP 5, where the errors with SCAN are fixed, in the 100 GPa C-AFM state band structure and spectral function calculations.

# S2 Details of electronic structures

## S2.1 Orbital-decomposed band structures and PDOSs

Figure 3 presents the orbital-decomposed electronic structures only for the most relevant orbitals ($Cu_{pl}$ $d_{x^2-y^2}$, $Cu_{pl}$ $d_{z^2}$ and $Cu_{ch}$ $d_{z^2}$). For completeness, in Figs. S2 and S3 we provide results for all orbital characters that have significant contributions in the displayed energy window.

We note that the zero-pressure G-AFM band structure presented in Fig. 3 (a) is very similar to the zero-pressure C-AFM band structure. Recall that the differences between the G-AFM and C-AFM states are only in the interlayer coupling which is not strong enough to substantially alter the band structure at low pressures.

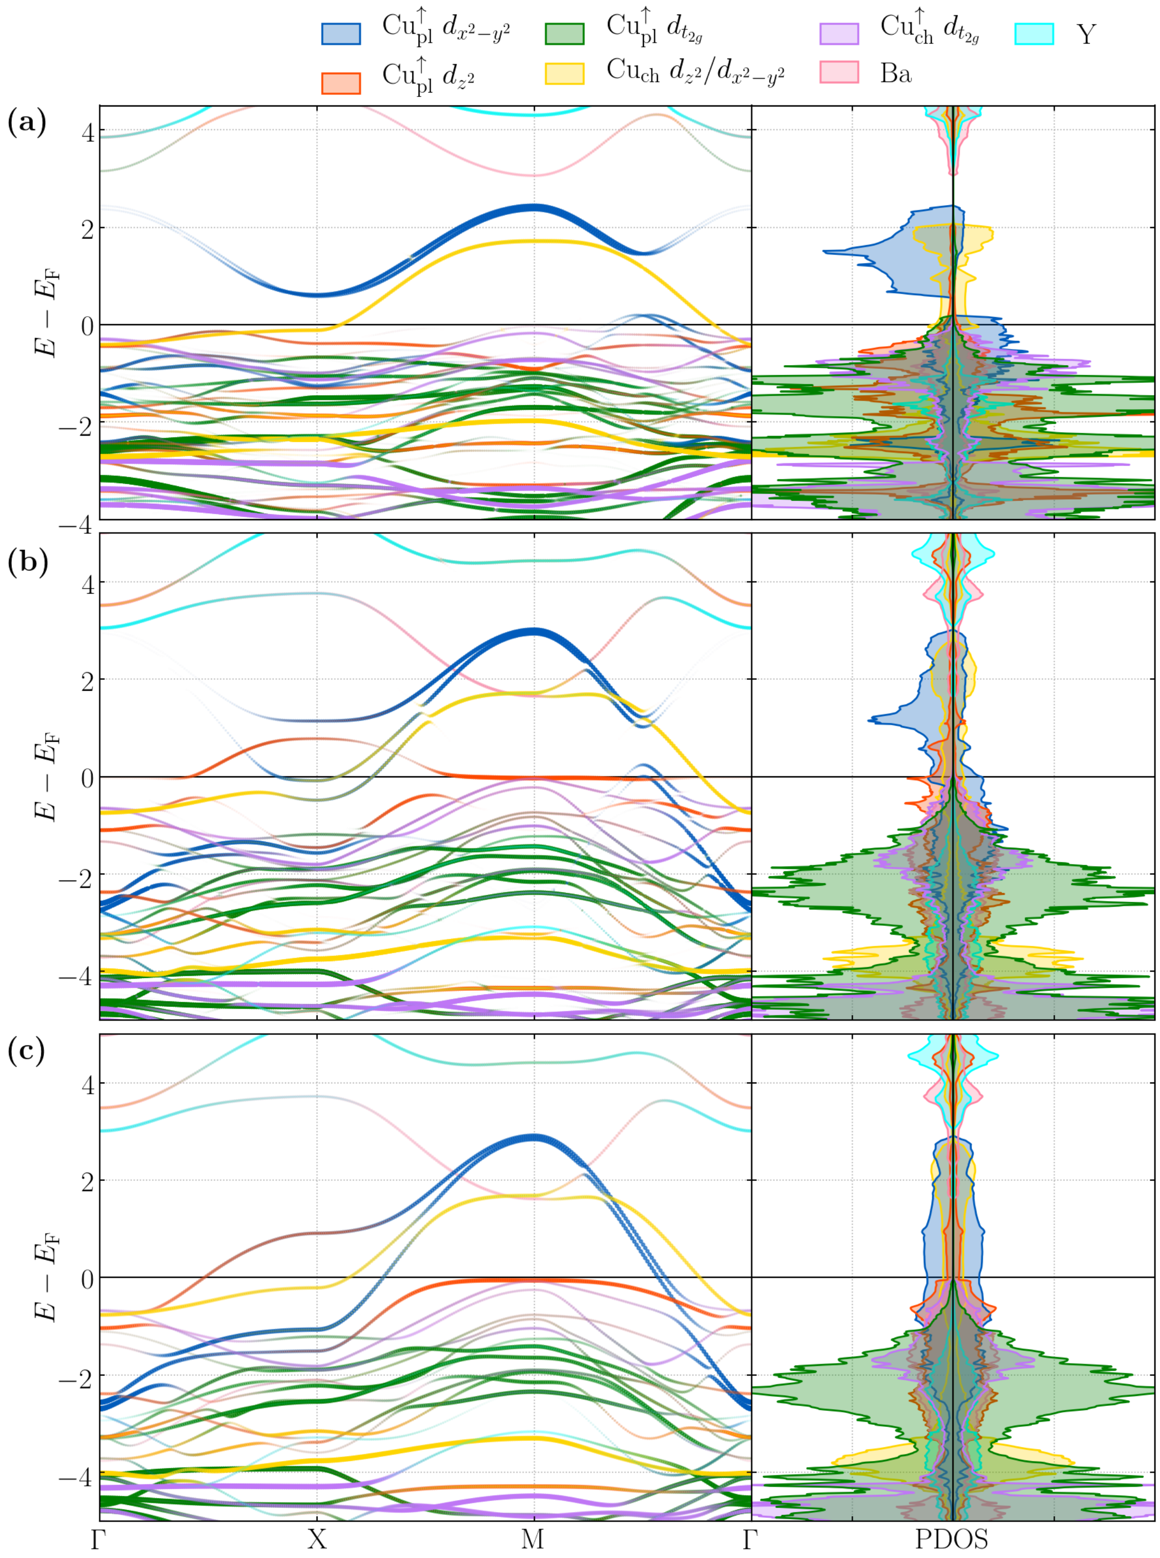


Figure S2: $YBCO_7$ band structure and PDOS projected for all Cu, Y and Ba orbitals that have significant contribution for (a): $P = 0$ G-AFM phase ($M = 0.462\,\mu_{\mathrm{B}}$), (b): 100 GPa C-AFM phase ($M = 0.326\,\mu_{\mathrm{B}}$) and (c): 100 GPa NM phase.

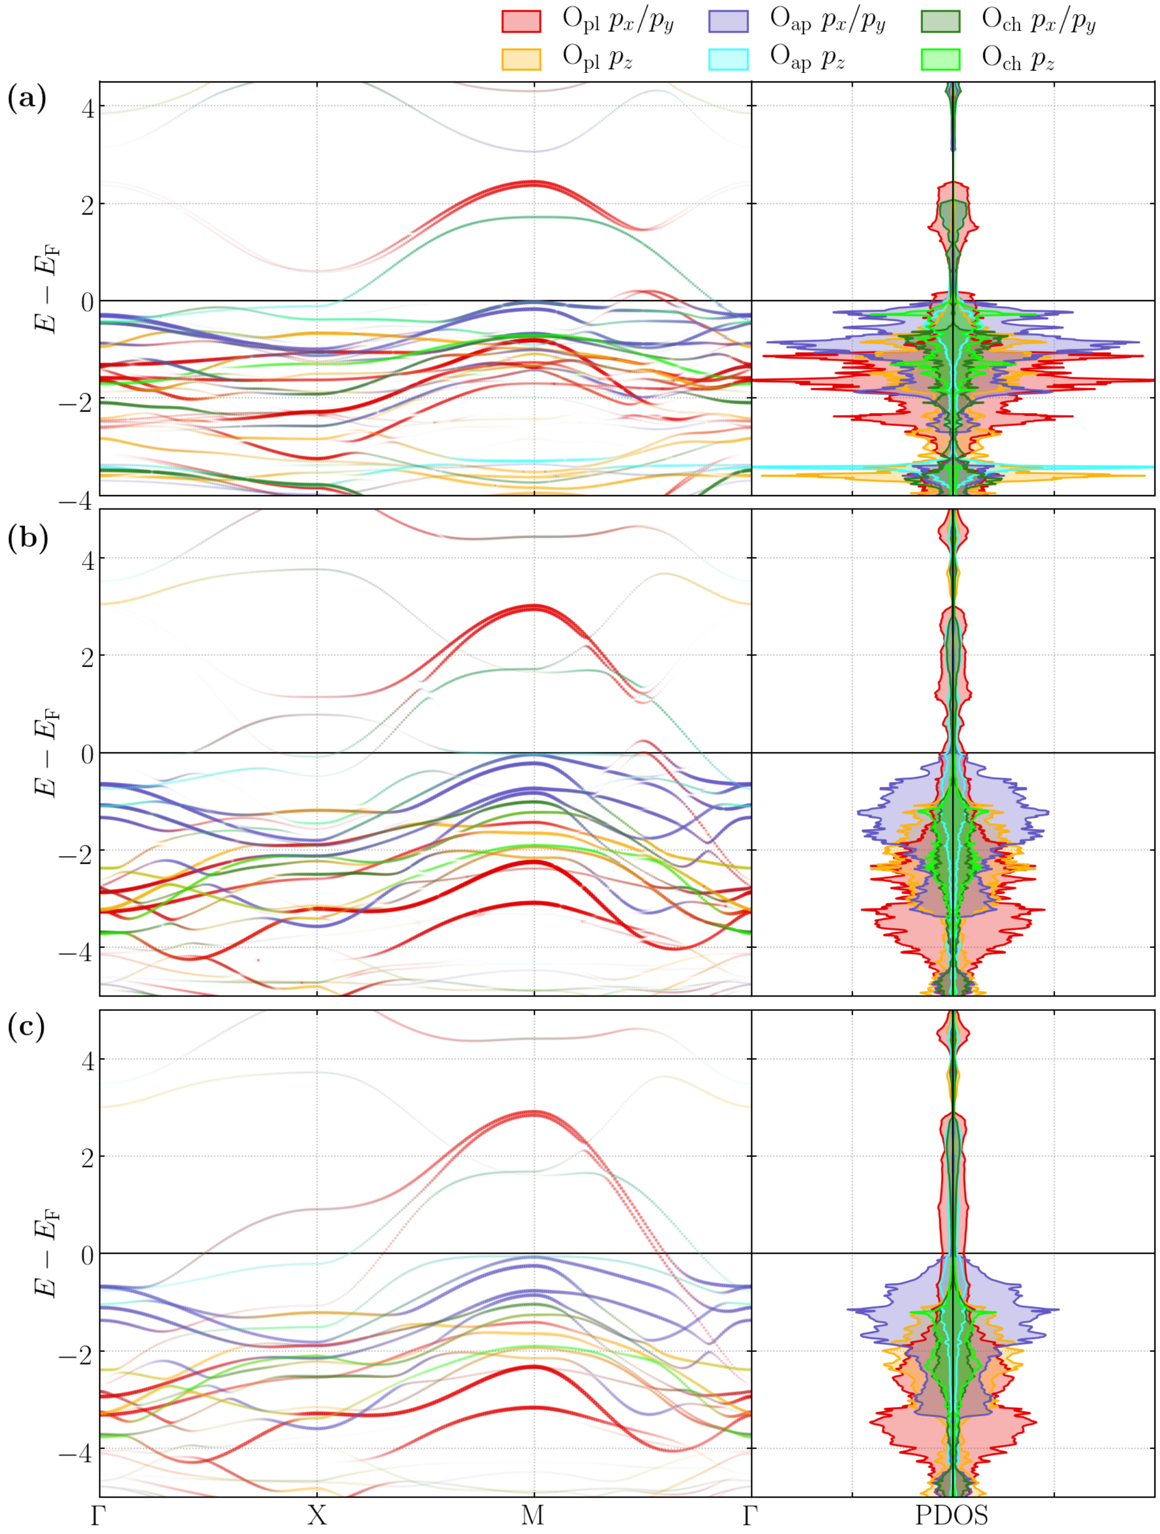


Figure S3: $YBCO_7$ band structure and PDOS projected for all oxygen orbitals that have significant contribution for (a): $P = 0$ G-AFM phase ($M = 0.462\,\mu_B$), (b): 100 GPa C-AFM phase ($M = 0.326\,\mu_B$) and (c): 100 GPa NM phase.

## S2.2 PDOS pressure evolution

To illustrate the transition of the electronic state under pressure more clearly, we present the pressure-evolution of the Cu PDOS for various magnetic states in Fig. S4.

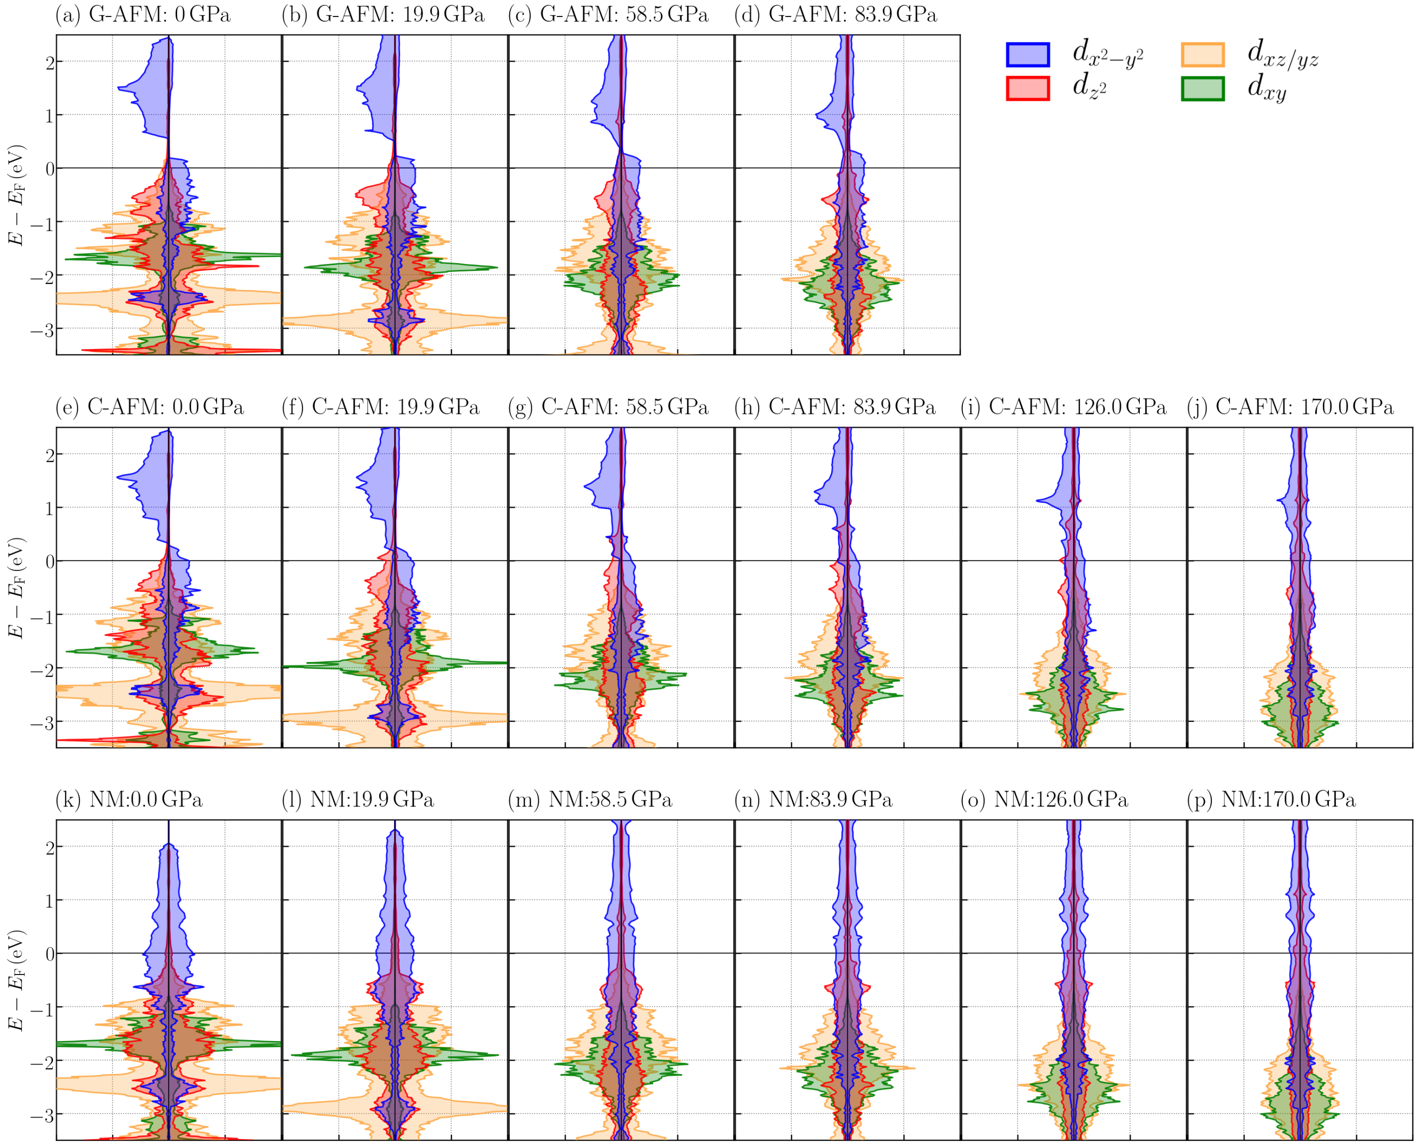


Figure S4: PDOS pressure-evolution for the G-AFM, C-AFM and NM magnetic configurations.

### S2.3 Three-dimensionality of the high-pressure electronic structure

Fig. S5 shows the NM band structure along high-symmetry $k$-paths at 100 GPa to highlight the slight high-pressure three-dimensionality of the electronic structure. Mainly, the Cu $d_{z^2}$ band is shifted downwards from the Fermi level. Also, the electronic structures along $\Gamma$–$X$–$M$ and $\Gamma$–$Y$–$M$ have differences in the CuO chain bands due to the orientation of the CuO chains. Note that the dispersion of the Cu $d_{z^2}$ band along the $M$–$R$ line leads to the emergence of two distinct van Hove singularities that move with respect to $E_F$ as a function of pressure.

## S3 Hole values

The hole contents presented in the main text Fig. 2 (a) are based on atomic charges calculated with the Bader charge analysis [46]. The Bader charges are obtained by integrating the charge density within the atomic volumes that are separated by isosurfaces of the electronic density gradient. To improve the accuracy of these calculations, we employed the charge partitioning algorithm [47], used dense real-space grids (Table S1), and averaged the calculated Bader charges over equivalent atoms in the unit cell.

The Bader analysis provides a robust method for determining the atomic charges and is considered reasonably accurate. Since it is space-filling, it has the advantage of being adaptable to naturally handle evolving structure and decreasing atomic volumes under pressure.

Hole contents in $YBCO_7$ were determined as differences in Bader charges with respect to $YBCO_6$ as the undoped base compound. Since $YBCO_6$ has strong G-AFM order even at room temperature, we used the Bader charge values for $YBCO_6$ G-AFM state as the reference for all the studied $YBCO_7$ cases (G-AFM, C-AFM and NM). $YBCO_6$ does not contain the chain oxygen atoms, therefore, we computed the charge states of the $O_{ch}$ atoms in $YBCO_7$ with respect to the isolated charge-neutral oxygen atoms.

### S3.1 Accuracy of the $CuO_2$ plane doping values

As discussed in the main text, the experimentally determined $CuO_2$ plane doping values are not equal to our ambient pressure Bader analysis results: we obtained $x = 0.11$, while the commonly accepted value for $YBCO_7$ is around 0.18, see for example Ref. [79]. However, it is challenging to establish full accord between the experimental and computational doping values for many reasons. Most importantly, the concept of doping in a real material is difficult to define exactly since the electrons are delocalized and there always is some charge density between the atoms that is difficult to strictly assign to any individual atom; it is not clear if some of this charge should be assigned to any atom at all, and thus, the experimental and theoretical interpretations of this charge are quite different. Experimentally, the doping values are determined via nuclear magnetic resonance (NMR) frequencies using the theoretical framework developed in Ref. [65]. Computationally, even though Bader analysis provides a robust and mathematically well-defined method for determining the atomic charges, as seen in our smooth doping

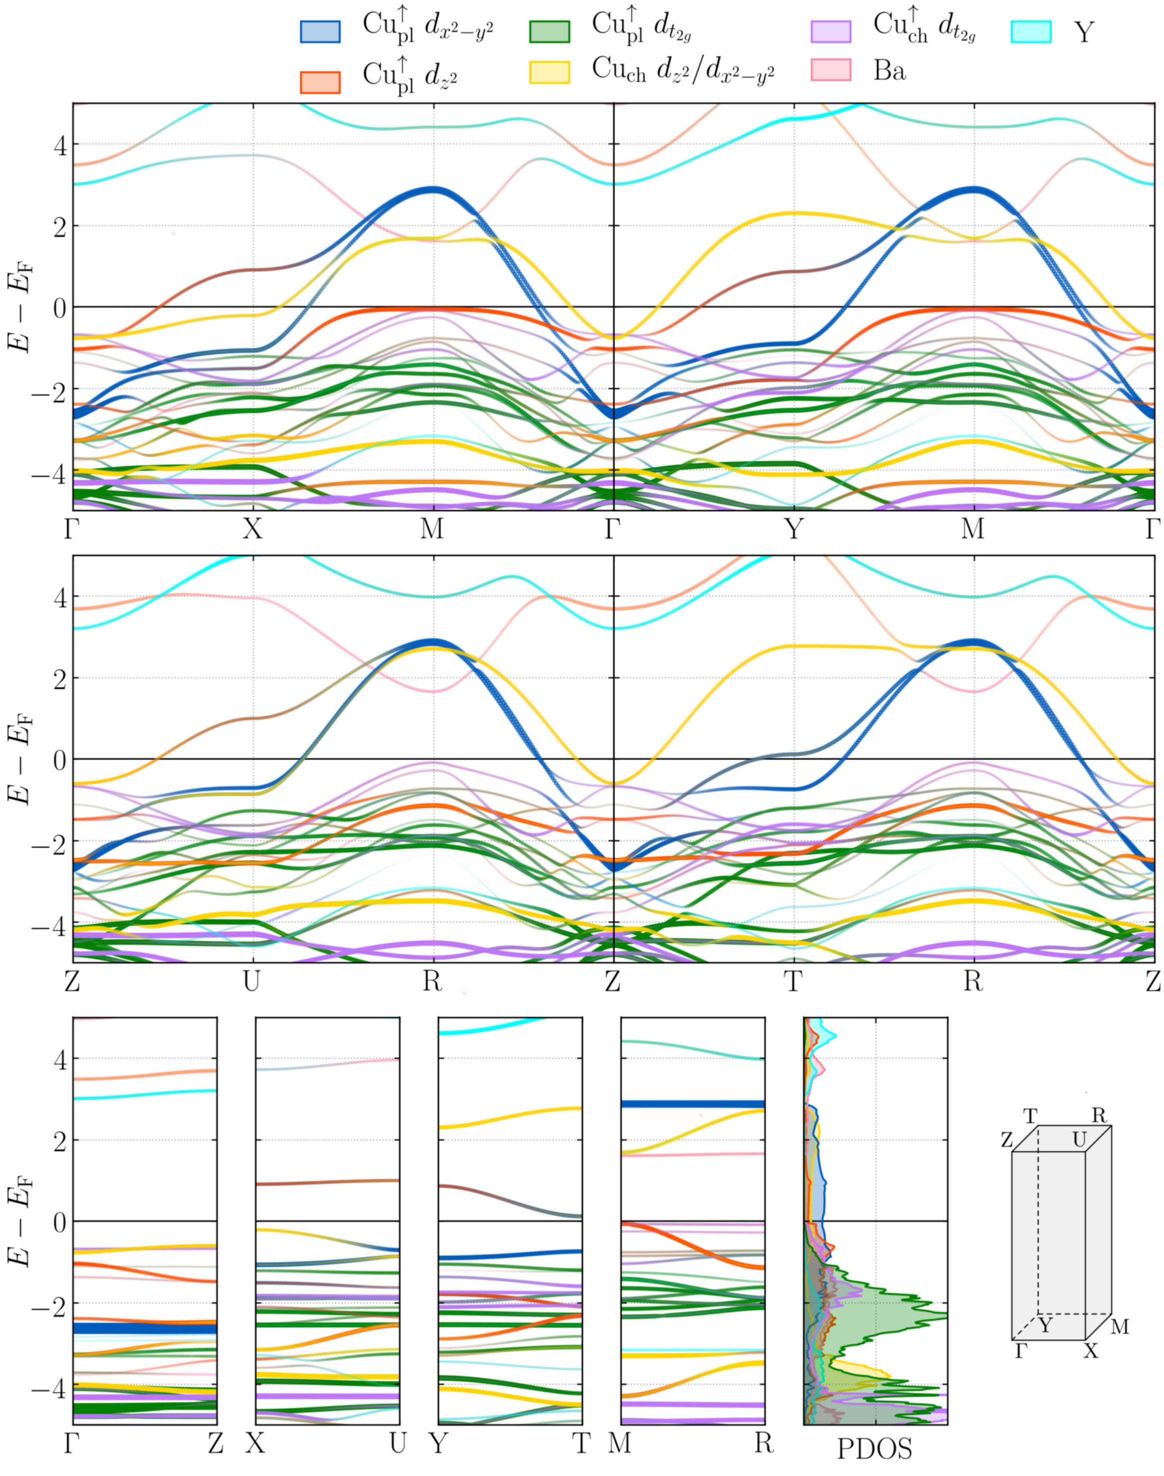


Figure S5: NM band structure at 100 GPa featuring various high-symmetry $k$-points: $\Gamma = (0,0,0)$, $X = (\frac{1}{2},0,0)$, $Y = (0,\frac{1}{2},0)$, $M = (\frac{1}{2},\frac{1}{2},0)$, $Z = (0,0,\frac{1}{2})$, $U = (\frac{1}{2},0,\frac{1}{2})$, $T = (0,\frac{1}{2},\frac{1}{2})$ and $R = (\frac{1}{2},\frac{1}{2},\frac{1}{2})$.

curves in Fig. 2 (a), it is probing a somewhat different quantity due to the ambiguities associated with the atomic volumes and the charges in the interstitial regions. For instance, our Bader analysis results clearly show that the apical oxygen atoms attain significant amount of doping (0.11 holes). If the $Cu_{pl}$ Bader volumes were extended to include some of the volume currently belonging to the $O_{ap}$ atoms, $CuO_2$ plane doping values around 0.18 could be obtained.

Despite the uncertainties in the absolute values of the $CuO_2$ plane doping, we expect our computed changes in doping due to pressure to be more robust. Our key finding is that the $CuO_2$ planes are strongly doped under pressure and that this doping originates from the Y and Ba ions.

## S3.2 Accuracy of the intraplanar charge transfer results

Our results regarding the intraplanar Cu–O charge transfer for relatively low pressures ($\lesssim 5\,\mathrm{GPa}$) are somewhat different from those in Ref. [64], where the pressure-dependence of $YBCO_{6+\delta}$ Cu and O hole contents was determined via NMR measurements: the authors observed a decrease in $x(\mathrm{Cu_{pl}})$ for their highest-doped sample ($YBCO_{6.9}$), while our results show a clear increase. However, the intraplanar charge is particularly challenging to determine with Bader analysis since the atoms are tightly packed and the electronic density is high, making the results sensitive to the choice of atomic volumes. The strong non-linearity of $x(\mathrm{Cu_{pl}})$ and $\tilde{x}_{\mathrm{pl}}^{\mathrm{O}}$ in our results indicates that there exist some non-trivial pressure effects in the local chemical environment of the $CuO_2$ planes. This makes sense since the covalency of the Cu–O bond is likely affected by the contraction of the lattice. The introduction of electrons with different orbital character ($d_{z^2}$) would further complicate the situation. These effects would most likely be accompanied with Cu–O charge transfer that might be probed differently by NMR experiments and Bader analysis. This suggests the importance of the Cu and O charge states in the physics of the second dome. Our Bader analysis results further suggest that the O hole content is important in the second dome regime, at least when the electronic structure is close to the second dome model of Ref. [8].

The non-monotonic changes of the oxygen hole fraction might be related to the changes in dimpling of the $O_{pl}$ atoms, see the blue curves in the main text Fig. 1 (d). The maximum in $x(\mathrm{Cu_{pl}})$ near $60\,\mathrm{GPa}$ in Fig. 2 (a) corresponds roughly to the observed disappearance of dimpling at $\sim 80\,\mathrm{GPa}$ ($\Delta z_{\mathrm{pl}} = 0$ in Fig. 1). If this is the reason for the behavior of the oxygen-hole fraction curve, this could mean that other cuprates may have distinctly different pressure-dependence for the oxygen-hole ratio since they do not feature as strong dimpling as YBCO.

## S3.3 Pressure-evolution of $Cu_{pl}$ orbital occupations

We present approximate orbital decomposition of the occupied $Cu_{pl}$ electrons in Fig. S6. These results are based on integration of orbital-decomposed PDOS, which are calculated from projections to hydrogen-like orbitals. The presented PDOS has been corrected by normalizing the values with respect to the $Cu_{pl}$ Bader charges as follows:

$$[\text{Orbital occupation}] = \int_{-\infty}^{E_\mathrm{F}} \mathrm{d}E\ [\text{Orbital PDOS}] \cdot \frac{[\mathrm{Cu_{pl}}\ \text{Bader charge}]}{\sum_\text{Orbitals} \int_{-\infty}^{E_\mathrm{F}} \mathrm{d}E\ [\text{Orbital PDOS}]}. \tag{1}$$

The corrective normalization was performed since the raw orbital-decomposed PDOS is obtained within the atomic spheres defined by strict radii (the `RWIGS` parameters in VASP). Bringing the atoms closer together with pressure alters the volumetric environments of the ions, which can even lead to atomic sphere overlap and thus to double-counting of orbital charge. The errors can be significant, as the total DOS-based electron count of the whole 26-atom system increases by several electrons in the studied pressure range. Adjusting the `RWIGS` parameter to account for these changes becomes both intricate and prone to errors, therefore, we performed the normalization with respect to the $\mathrm{Cu_{pl}}$ Bader charge that is robust to pressure effects. However, the errors are difficult to fully eliminate even with this method since the projections to the pure hydrogen-like orbitals do not always properly capture the strongly hybridized molecular orbitals. Normally integrating the PDOS of given orbital symmetry over the full energy range (considering both occupied and unoccupied electrons) should give a result close to 2.0 (or 1.0 if spin is not considered). This is not the case for example for $\mathrm{Cu_{pl}}$ $4s$. As shown in Fig. S6, the $4s$ orbital is captured in the PDOS integration only weakly even though it is nominally occupied: it also does not properly show up in the unoccupied part of the PDOS. This skews the normalization factor in Eq. (1) for all orbitals since the $4s$ electrons are properly taken into account in the Bader charge but not in the PDOS-integrated charge. However, we believe that our analysis provides a reasonable picture of the development of orbital occupancies under pressure.

As discussed in the main text, the $\mathrm{Cu_{pl}}$ $d_{z^2}$ orbitals lose occupation (gain holes) under pressure as the $\mathrm{Cu_{pl}}$ $d_{z^2}$ bands rise to the Fermi level. Figure S6 quantifies this effect. Concurrently, the occupation of $\mathrm{Cu_{pl}}$ $d_{x^2-y^2}$ stagnates as a function of pressure and even increases at high pressures. Thus the ratio between the $\mathrm{Cu_{pl}}$ $d_{z^2}$ and $d_{x^2-y^2}$ holes develops drastically in the favor of $d_{z^2}$, which might have important consequences for the second dome physics. Interestingly, the $d_{t2g}$ holes also increase under pressure, indicating that even more complex multi-orbital models than the $d_{z^2}$—$d_{x^2-y^2}$ models might be needed. It is notable that the $p$ and $s$ orbitals also receive electrons under pressure, explaining the observed negative high-pressure excursion in the $\mathrm{Cu_{pl}}$ hole content discussed in Fig. 2 (a).

## S3.4 Pressure-evolution of orbital contributions to the magnetic moment

Using the same methodology as that used for the orbital-occupation computations above, we have calculated the approximate orbital contributions to the $\mathrm{Cu_{pl}}$ magnetic moments (Fig. S7). As expected, the unpaired $d_{x^2-y^2}$ orbital contributes the majority of the magnetic moment at all pressures. This contribution steadily decreases as a function of pressure even though the total $d_{x^2-y^2}$ orbital occupations remain roughly constant, which is due to the flattening of the $d_{x^2-y^2}$ PDOS (Fig. S4). The $d_{z^2}$ orbitals only provide a marginal contribution at zero pressure but, interestingly, under pressure the contribution starts to increase, especially for the C-AFM case. Around the proposed second dome ($P = 100\,\mathrm{GPa}$) this contribution is about 25 % to the magnetic moment and at higher pressures it is even greater. This result emphasizes the significant role of the $d_{z^2}$ orbitals near the proposed second dome.

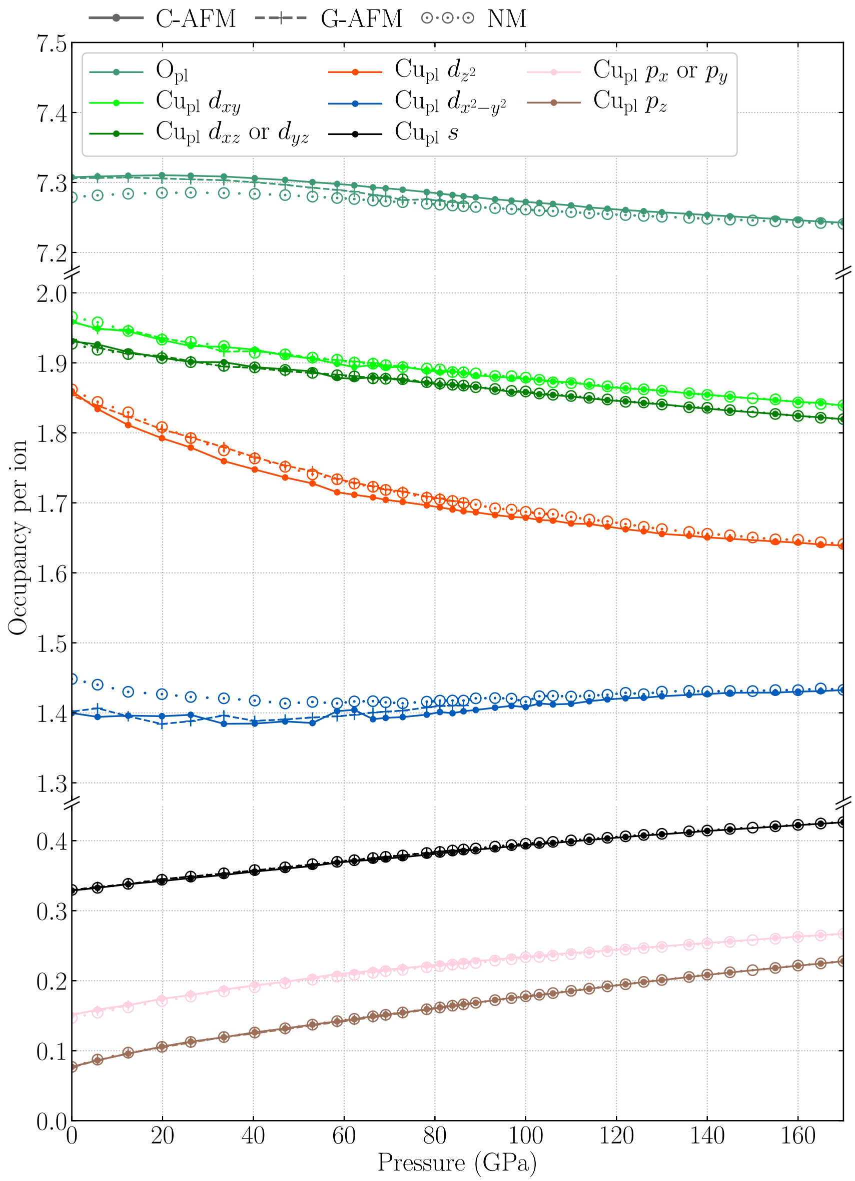


Figure S6: Approximate orbital occupations related to the $Cu_{pl}$ ion. Bader charge for the planar oxygen ion, which is directly related to the hole content $x(O_{pl})$ in the main text Fig. 2 (a), is also plotted for comparison.

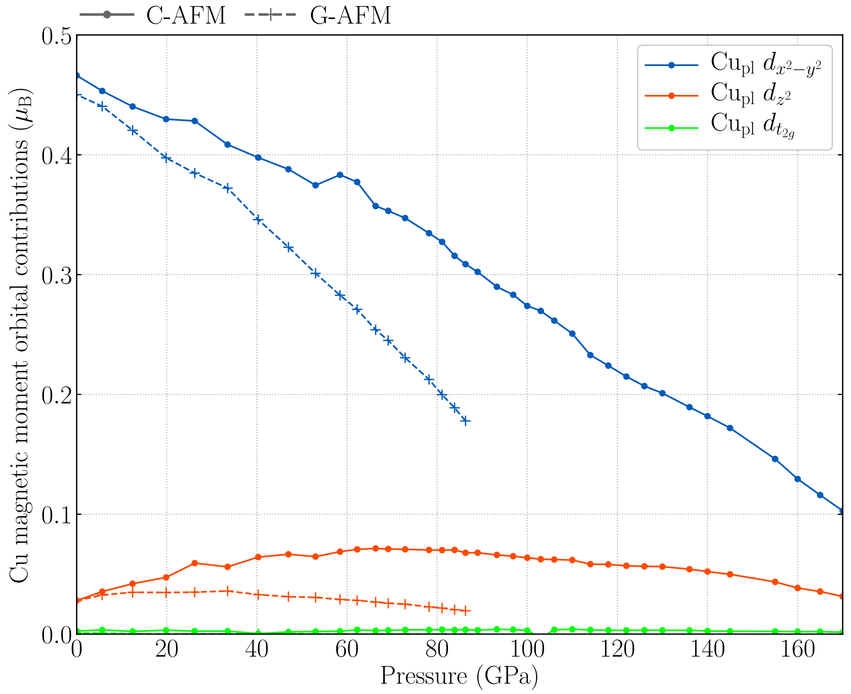


Figure S7: Approximate orbital contributions to the $Cu_{pl}$ magnetic moments.

# S4 Stripe phases

We have also considered magnetic stripe phases since stripe phases with large periodicities were found to be the true ambient-pressure ground state in $YBCO_7$ in our earlier work [36]. However, due to the computational complexity of the high-pressure calculations outlined above, we were not able to explore stripe phases with as large supercells as in the zero-pressure case. Therefore, we limited our study to $3 \times 2$ and $2 \times 3$ supercells, which are three times larger than the $\sqrt{2} \times \sqrt{2}$ G/C-AFM supercell.

As a first step, we performed preliminary tests with a soft oxygen potential to find the most stable small-supercell stripe phase at moderate ($\lesssim 20$ GPa) pressures, where the errors due to the soft potential still are negligible. We tested both the bond-centered and site-centered phases with different magnetic interlayer couplings, see Fig. S8. We found the $3 \times 2$ supercell phases to be in general more stable than the $2 \times 3$ ones. The most stable of the studied phases was the $3 \times 2$ supercell bond-centered stripe with C-AFM-type interlayer coupling [Fig. S8 (a)]. We selected this phase for a detailed pressure study with hard oxygen potentials. As shown in the main text Fig. 2 (b), increasing pressure destabilizes this phase ("B-stripe") rapidly; its enthalpy plateaus between $\sim$ 50–70 GPa as it goes through a gradual transition into the site-centered stripe phase with G-AFM-type interlayer coupling ["S-stripe", Fig. S8 (b)]. This transition is evident at 60 GPa, where the Cu magnetic moments are a linear combination of these two stripe phases.

The magnetic moments shown in the main text Fig. 2 (b) are averaged over all $Cu_{pl}$ sites, so that the sites with zero magnetic moments in the S-stripe contribute to the average. Interestingly, these averaged

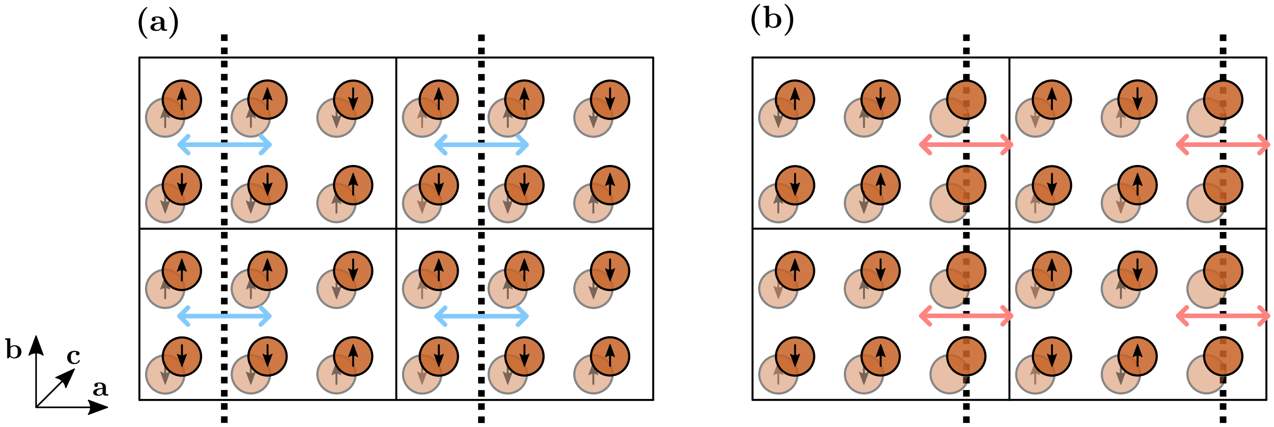


Figure S8: Examples of stripe phases in the bilayer $CuO_2$ network. Magnetic moments of the Cu ions (brown circles) are marked with arrows and the O ions are not pictured for clarity. The lower $CuO_2$ layer is drawn with fainter color and the $3 \times 2$ supercell is marked with solid line. (a): A bond-centered stripe with G-AFM-type interlayer coupling. The stripe inversion plane (dashed line and blue arrows) is located at the bonding oxygen site. The Cu sites next to the inversion plane are forced to have parallel spins. (b): A site-centered stripe with C-AFM-type interlayer coupling. The stripe antiphase boundary (dashed line and red arrows) is located at Cu sites with zero magnetic moments. The periodicity of these phases is three in the $a$-direction. Since the CuO chains are aligned along the $b$-axis, they can be thought of as $a$-direction stripes with a periodicity of two.

magnetic moments for both phases follow the G-AFM phase magnetic moments as a function of pressure. Curiously, for this stripe phase the interlayer coupling transitions from C-AFM to G-AFM type under pressure, while in the minimal magnetic unit cell the transition is from G-AFM to C-AFM type. Note that stripe phase transitions with pressure are expected, as changes in the Fermi surface with doping lead to changes in the stripe nesting vectors. This mechanism may be at play in the phase transitions recently observed in Ref [22]. Similar stripe phenomena have been found in the superconducting nickelates [39].

# S5 Theoretical considerations concerning the second dome

## S5.1 Pseudogap physics and the second dome

Progress in resolving the origins of superconductivity in the cuprates has been hampered by a lack of understanding of their normal states. In particular, the role of the pseudogap phenomenon has been a longstanding problem. The pseudogap is an anomalous gap in the normal-state energy spectrum, which exists in the cuprate phase diagram above $T_c$. While the nature of the pseudogap phase remains controversial, it is widely believed to be composed of intertwined AFM and stripe/charge-density wave (CDW) orders [69,70]. The pseudogap disappears at a critical doping value $x^*$, which is known as the pseudogap collapse. Recent experiments have elucidated the phenomenology of pseudogap collapse in

overdoped cuprates in considerable detail [69–72]. Notably, at atmospheric pressure, the competing charge stripe orders disappear shortly before the pseudogap collapses. Surprisingly, many features of this collapse also seem to mirror the phase transition in an ordinary antiferromagnet [73].

Recent first-principles DFT calculations [36,40] have shed considerable light on the pseudogap in $YBCO_7$, finding that a number of magnetic and stripe phases are nearly degenerate in energy, and that the organizing principle for these phases is local moment formation. This is consistent with a picture in which the long-range AFM order is missing in the pseudogap phase, while the short-range magnetic coupling persists, reflecting pseudogap physics [73]. An important prediction of the model is that when the AFM phase disappears it takes its topological defects with it. That is, the stripe phases should disappear at approximately the same doping as the AFM phase [73,75].

$YBCO_7$ is known to be in the pseudogap phase, but close to its collapse [76], We therefore expect that a relatively small increase in pressure-induced hole doping of the $d_{x^2-y^2}$ orbitals would eliminate the AFM and stripe orders to reveal the physics of the collapse and the resulting new ground state. However, it turns out that pressure introduces entirely new physics: by reducing the difference between the $c$ and $a$ axis, a new channel for doping ($d_{z^2}$) opens up while the $d_{x^2-y^2}$ channel becomes less significant with its occupation being essentially unaffected by pressure (see Fig. S6). This mechanism seems to preserve the $d_{x^2-y^2}$-pseudogap (magnetic and charge order) to much higher pressure-doping values compared to the case of chemical doping. In fact, the observed stabilization of the NM ground state near 100 GPa has much in common with the conventional cuprate pseudogap collapse with doping. As noted above, stripe phases are also found at high pressures, and at the pressure-induced transition near 100 GPa all magnetic phases become unstable at nearly the same pressure. It should be noted, however, that our demonstration is incomplete, since we are unable to calculate stripes with larger charge periodicity, which are known to include the $YBCO_7$ ground state at low pressures.

Our analysis suggests that the pseudogap collapse occurs when the AFM van Hove singularity (VHS) crosses the Fermi level [73]. Figure S4 presents a detailed pressure evolution of the $Cu_{pl}$ PDOS. It shows that in the C-AFM phase, a $d_{x^2-y^2}$ VHS appears to be pinned near the Fermi level from 0 to 126 GPa, while a $d_{z^2}$ VHS moves steadily towards $E_F$ between 58.5 and 126 GPa. At higher pressures, both VHSs move above the Fermi level, and the spin-up – spin-down differences become weak. In the NM phase a $d_{z^2}$ VHS smoothly rises with pressure, crossing the Fermi level near 126 GPa. The main text Fig. 2 further shows that the stripe phase magnetic moment extrapolates to zero near 120 GPa. Thus, the transition appears to be a two-step process, with the NM phase becoming lower in energy near 90 GPa, while the $d_{z^2}$ VHS crosses the Fermi level near 126 GPa, possibly associated with the larger-periodicity stripe phases.

The aforementioned stabilization of a NM phase is quite similar to the doping-induced pseudogap collapse found in the cuprates, where a two-step transition is often found, with the charge order disappearing at a lower doping than pseudogap (short-range AFM order) collapse, see Ref. [73] and references therein. By studying the integrated magnetic neutron scattering spectra in LSCO, where the pseudogap collapses near $x^* = 0.2$ [80], it has been shown that at $x = 0.25$ only isolated magnetic islands are present [74], that are likely associated with doping inhomogeneity [81]. At $x = 0.3$, no magnetic fluctuations are found below 60 meV [74]. Notably, here by using pressure to dope the system, we have minimized effects of

doping-related heterogeneity. A similar pressure-induced pseudogap collapse, from small to large Fermi surface, has been observed in an iron-based superconductor [18] that is associated with a transition to a second superconducting dome.

### S5.2 Spin fluctuations and $s^{\pm}$ superconductivity

In addition to the surprising persistence of the pseudogap to high pressures, it is also surprising that the C-AFM phase persists as a metastable state over the entire pressure range. In this connection, the possibility of $s^{\pm}$ superconductivity triggered by spin fluctuations in correlated materials including second dome physics has been discussed in the literature [4–6,8,12,14]. In particular, Ref. [12] discusses the difference between pair-breaking and pair-forming fluctuations and suggests that the optimal pair-forming fluctuations occur around $0.1|t|$ or $\sim$ 65 meV for $YBCO_7$, see Sec. S7 for the value for the hopping parameter $t$ at high pressures. The evolution of PDOS in Fig. S4 shows that the PDOS peaks related to the $d_{z^2}$ flat band go through the Fermi level near 120 GPa and can be tuned to the 65 meV range by correct pressure, optimizing pair forming spin fluctuations around 100 GPa (peak below $E_{\mathrm{F}}$) or 170 GPa (peak above $E_{\mathrm{F}}$). Notably, the oxygen orbital character in the main text Fig. 4 is found to be large in this pressure range.

## S6 Lattice stability of $YBCO_7$ under pressure

Some experiments indicate lattice parameters to deviate from the expected equation of state under pressure [43] and even show signs of structural instabilities [44]. As shown in the main text Fig. 1 (d), we did not find any such irregularities under pressure. Our structure, however, is perfectly stoichiometric since there are no CuO chain defects. Therefore, the experimental lattice parameter deviations in $YBCO_{7-\delta}$ ($\delta > 0$) could be caused by transitions within the stripe phases or reordering of the incomplete CuO chains observed in other studies [51,52], especially since these phenomena are observed in the same pressure range (below 20 GPa).

Since our calculations involve very high pressures, we have calculated the phonon spectrum of $YBCO_7$ at 100 GPa in search of soft phonon modes that would indicate structural instabilities. The phonon calculations were performed using the finite-differences approach implemented in VASP and invoked by setting `IBRION = 6` and `LPHON_DISPERSION = TRUE`. The used supercell was obtained by repeating the 13-atom NM primitive cell $2 \times 2 \times 2$ times. We used total energy tolerance of $10^{-8}$ eV and atomic force tolerance of 0.01 eV/Å when relaxing the initial structure since the finite differences approach requires high accuracy, see Sec. S1.1 for the real and $k$ space grids used. For each of the 30 degrees of freedom two atomic displacements were considered and the total energy calculation was performed. The displacements were set to a small value of 0.003 Å since at high pressures even small perturbations lead to large forces that could become non-harmonic.

We performed the calculations at 100 GPa and to reduce the computational cost we considered the NM

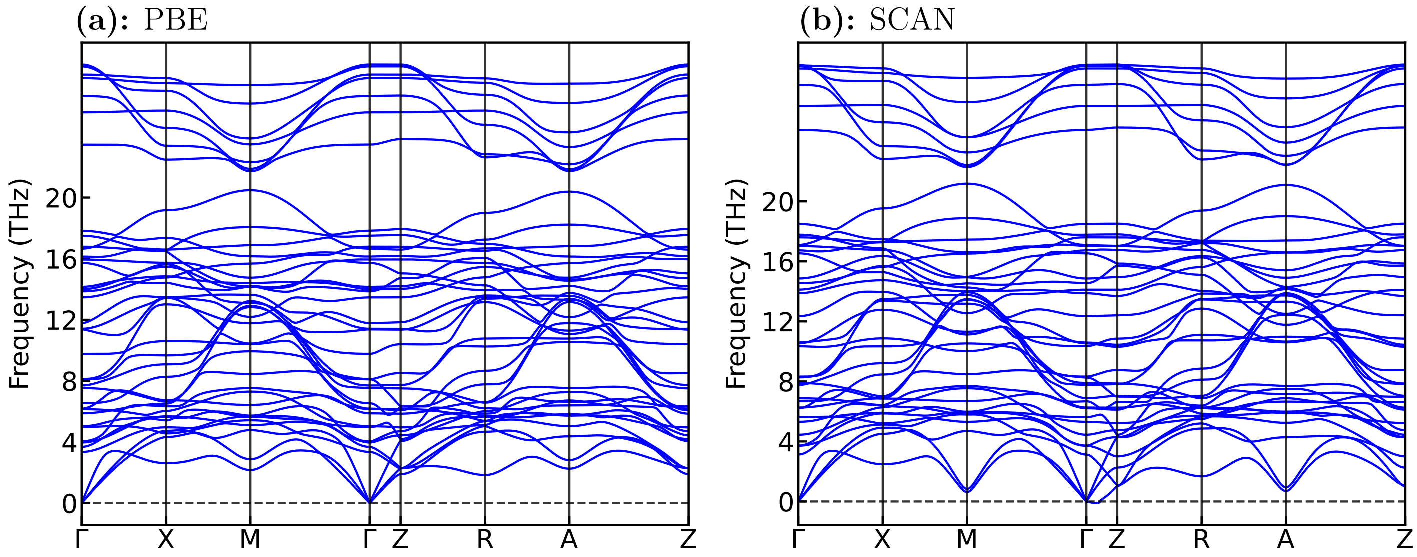


Figure S9: Phonon dispersion in NM $YBCO_7$ at 100 GPa for (a) PBE and (b) SCAN.

phase since magnetism is not expected to affect the structural stability at high pressures. We used both PBE and SCAN functionals. The resulting phonon spectra are shown in Fig. S9. The PBE and SCAN results are seen to be quite similar which is not surprising since the main improvements of SCAN over PBE in YBCO are in the description of the electronic correlations in the $CuO_2$ planes and in the handling of the weak bonding across the van der Waals gaps. The electronic states only induce relatively small effects on the phonons when the layers are squished together under pressure, and the subtleties of the layer-layer interactions across the van der Waals gaps become less important than the simple Coulomb repulsion effects.

Our results in Fig. S9 do not feature signs of instabilities (negative-frequency branches). However, the SCAN result displays a flat zero-frequency band along the $\Gamma$–$Z$ line, probably because we did not use a dense enough $k$-point grid for the SCAN calculation: based on our previous experience on phonon calculations, SCAN is particularly sensitive to the $k$-point grid density. Our SCAN calculations were computationally very expensive, so we did not repeat the calculations for a denser grid, but we believe that for an appropriately denser $k$-point grid, the SCAN results along the $\Gamma$–$Z$ line would converge towards the PBE result, as is the case with the 100 GPa NM electronic structure (Fig. S1).

# S7 Tight binding model

To better understand hybridization effects in the electronic structure of the NM high-pressure phase, we fitted our first-principles band structure to a minimal tight-binding model. A four-band model previously applied to the manganites [57] was found to give an excellent fit that captures the salient features of the NM YBCO phase at 0 GPa and 100 GPa near the Fermi level. This model neglects the chain Cu and inter-cell hopping along the $c$-axis, along with the effects of orthorhombicity of the YBCO

structure. The fit's accuracy justifies these approximations. To allow comparison of our model with the model of Maier *et al*'s [8], we rescaled some terms in the Hamiltonian in relation to the formulation of Ref [57].

Our four-band model with intra-orbital symmetric (+) and anti-symmetric (−) basis, decouples into two block diagonal $2 \times 2$ Hamiltonians, $H_{\pm}$:

$$H_{\pm} = \begin{pmatrix} H_{11} + E_z/2 \pm t_{bi1} & H_{12} \\ H_{12} & H_{22} - E_z/2 \pm H_{bi2} \end{pmatrix} \tag{2}$$

where $H_{ij}$ and $H_{bi2}$ refer to

$$\begin{aligned} H_{11} &= 2t_{11}[c_x(a) + c_y(a)] + 4t'_{11}c_x(a)c_y(a) + 2t''_{11}[c_x(2a) + c_y(2a)] + 2t'''_{11}[c_x(3a) + c_y(3a)], \\ H_{22} &= 2t_{22}[c_x(a) + c_y(a)] + 4t'_{22}c_x(a)c_y(a), \\ H_{12} &= 2t_{12}[c_x(a) - c_y(a)] + 4t'_{12}[c_x(2a) - c_y(2a)] + 2t''_{12}[c_x(2a)c_y(a) - c_x(a)c_y(2a)], \\ H_{bi2} &= t_{bi2} + t'_{bi2}[c_x(a) + c_y(a)]/2. \end{aligned} \tag{3}$$

Here subscripts 1 and 2 refer to the $d_{x^2-y^2}$ and $d_{z^2}$ orbitals respectively. The $t_{ij}$ terms are the intra-planar hopping parameters between the $i$ and $j$ orbitals and $t_{bii}$ terms represent the inter-planar hopping parameters between the $i$ orbitals. The $c_i(\alpha a)$ terms represent $\cos(k_i \alpha a)$ with $i$ as either $x, y$ and $\alpha$ an integer value. $E_z$ is a crystal-field-splitting parameter to characterize the energy difference between the $d_{x^2-y^2}$ and $d_{z^2}$ orbitals and a chemical potential $\mu$ is included to match the Fermi level between the model and the first principles results.

While the three highest energy bands are easily distinguished by their strong $d_{x^2-y^2}$ and $d_{z^2}$ character [Fig. 3 (c)], the lowest energy band is distorted due to hybridization with other Cu $d$ orbitals not considered in our minimal model. Due to the uncoupling of the $d_{x^2-y^2}$ and $d_{z^2}$ orbitals along the nodal direction, $\Gamma - M$, we fitted the $t_{22}$, $t'_{22}$, $t_{bi2}$ and $t'_{bi2}$ parameters algebraically to minimize the effect of these other orbitals on our fit near the Fermi level. The energy values used in the algebraic equations are shown as black diamonds in Fig. S10. The remaining TB parameters were fit using a least squares algorithm. The TB parameters for 0 GPa and 100 GPa are given in Table S2, while the bands are shown in Fig. S10.

It is possible to map our symmetric Hamiltonian $H_+$ to the Hamiltonian in Ref. [8] up to the next-nearest neighbor terms. In our model, the crystal-field-splitting term $E_z$ and the nearest-neighbor bilayer splitting terms $t_{bi1}$ and $t_{bi2}$ play the role of the $d_{x^2-y^2}$ and $d_{z^2}$ on-site energies. The next-nearest-neighbor bilayer splitting term $t'_{bi2}$ can be combined with the $t_{22}$ to create an effective hopping term $t^{\text{eff}}_{22}$. In this way, the addition of bilayer splitting only serves to modify the on-site energy and the intralayer hopping.

By comparing the $H_+$ bands at 100 GPa with those of Ref. [8] at a doping of $x = 0.85$, it can be seen

that the electronic structure at 100 GPa is doped slightly less, with the $d_{z^2}$ band just breaking into the Fermi surface at the $M$ point. By using the connection between our model and that of Ref. [8], we can extract the doping level for $YBCO_7$ at 100 GPa. In Ref. [8], the on-site energy of $d_{x^2-y^2}$ is kept fixed at $\varepsilon_{d_{x^2-y^2}} = -0.222$ and the on-site energy of $d_{z^2}$ varies as $\varepsilon_{d_{z^2}}(x) = 0.661 - 5(1-x)$. As the on-site energies in $H_+$ are equal to $\varepsilon_{d_{x^2-y^2}} = E_z/2 + t_{bi1}$ and $\varepsilon_{d_{z^2}} = -E_z/2 + t_{bi2}$, we can shift them by the difference, $-0.222 - E_z/2 - t_{bi1}$, to fix the on-site energies between our model and that of Ref. [8]. By solving for the doping level $x$ with the TB parameters at 100 GP, we find that $x = 0.75$, which sits around the edge of the underdoped side of the second dome predicted in Ref. [8].

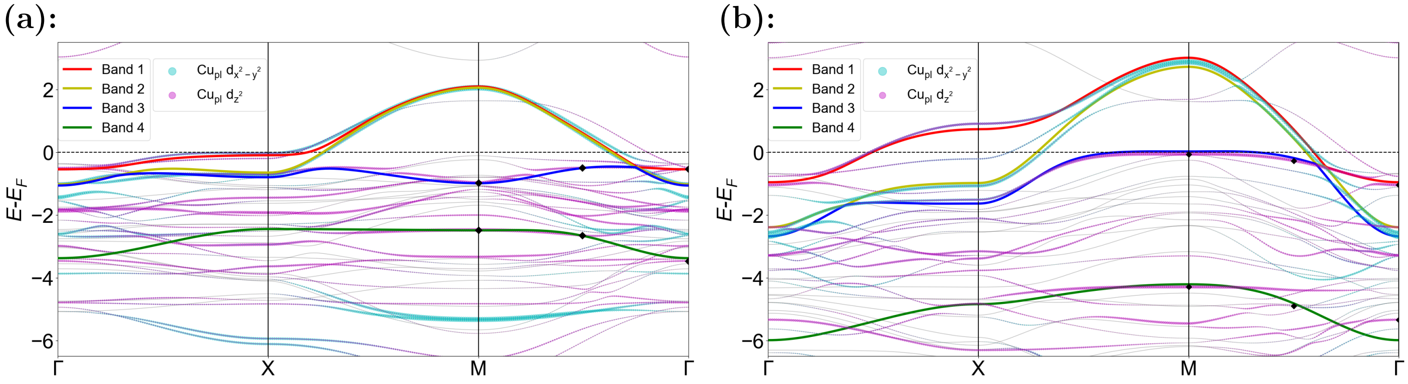


Figure S10: Electronic structure of $YBCO_7$ determined using DFT at (a) $P = 0$ GPa and (b) $P = 100$ GPa, in thin gray lines with planar $Cu_{pl}$ $d_{x^2-y^2}$ (cyan) and $d_{z^2}$ (magenta) weights overlaid. The size of the dots is proportional to the weights. The bands as fit by the TB model are plotted on top of the underlying DFT electronic structure. The black diamonds represent the energy levels chosen to algebraically solve for several tight binding parameters.

Table S2: Tight binding parameters (in eV) calculated for the NM $YBCO_7$ phase at $P = 0$ GPa and $P = 100$ GPa.

| P (GPa) | $t_{11}$ (eV) | $t'_{11}$ (eV) | $t''_{11}$ (eV) | $t'''_{11}$ (eV) | $t_{12}$ (eV) | $t'_{12}$ (eV) | $t''_{12}$ (eV) |
|---|---|---|---|---|---|---|---|
| 0 | −0.374 | 0.149 | −0.082 | −0.016 | −0.094 | 0.006 | −0.012 |
| 100 | −0.650 | 0.164 | −0.134 | −0.025 | −0.296 | −0.016 | −0.017 |
| P (GPa) | $t_{22}$ (eV) | $t'_{22}$ (eV) | $t_{bi1}$ (eV) | $t_{bi2}$ (eV) | $t'_{bi2}$ (eV) | $E_z$ (eV) | $\mu$ (eV) |
| 0 | −0.028 | −0.066 | 0.018 | 1.083 | 0.332 | 1.833 | 0.669 |
| 100 | −0.173 | −0.071 | 0.144 | 2.315 | 0.200 | 2.545 | 1.228 |

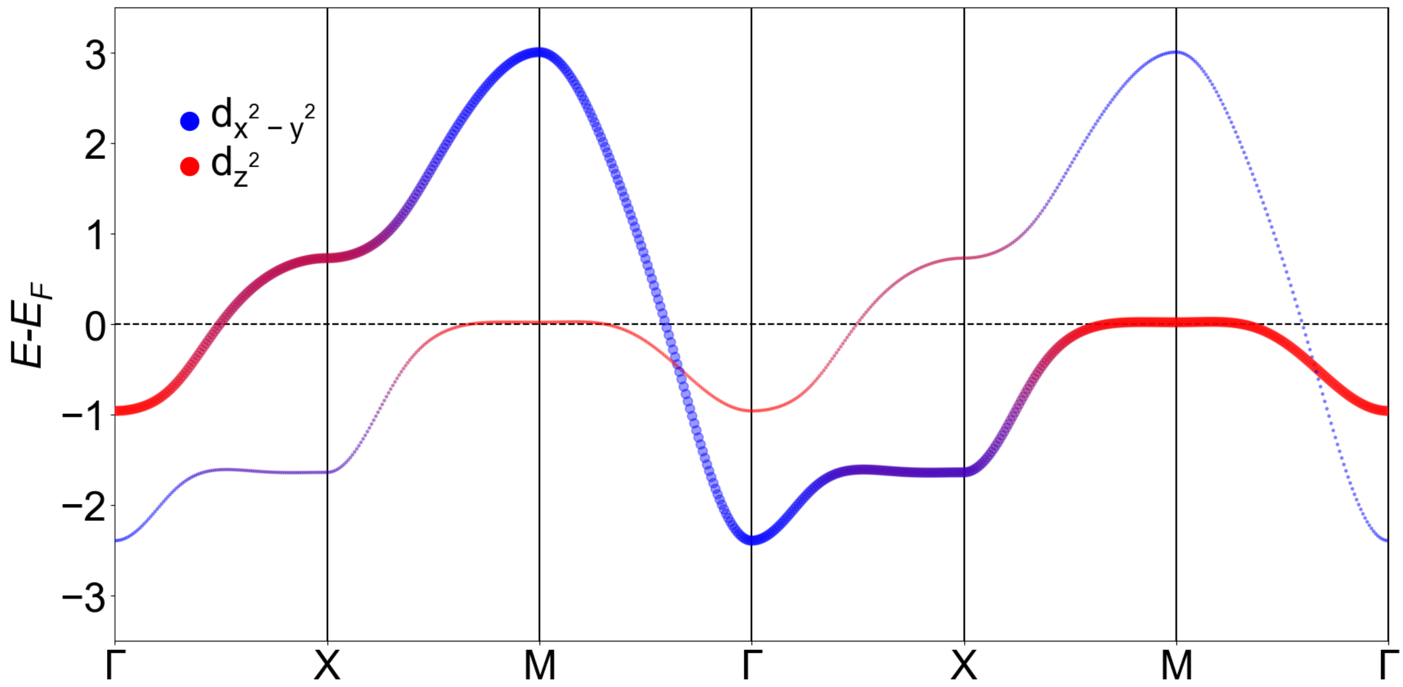


Figure S11: Plot of the $H_+$ bands along the $\Gamma \to X \to M \to \Gamma \to X \to M \to \Gamma$ path. The band character associated with the energy level is represented by the color of the k-point. The Möbius band is highlighted with stronger weight to show how one must travel around the path twice to reach the original energy level.

### S7.1 Möbius band

We observe an interesting consequence of the momentum-dependent hybridization of the $H_+$ bands. Along the $\Gamma \to X$ path the $d_{x^2-y^2}$ and $d_{z^2}$ bands hybridize and anticross. However, along the $\Gamma \to M$ path, $H_{12} = 0$ for all $k_x = k_y$ (see Eq. 3), which leads to the bands crossing without hybridizing along this path. This can also be understood with a symmetry argument: the $\Gamma$–$M$ line is a mirror plane and $d_{x^2-y^2}$ and $d_{z^2}$ have opposite parities and cannot interact. This leads to the curious result that if one starts at the higher energy $H_+$ band at $\Gamma$ and continuously follows the band character along the $\Gamma \to X \to M \to \Gamma$ path one returns to the lower energy $H_+$ band at $\Gamma$. In analogy to the mathematical object, the Möbius strip, if one follows the band characters along this path one more time they return to the original starting point of the higher energy band. This behavior is exemplified in Fig S11 where the $H_+$ energies along the above path are highlighted. This behavior is also present in the DFT bands, as seen in Fig. 3 (c), but it is complicated by additional splittings caused by hybridizations not included in our minimal model (e.g. chain Cu and planar Cu $t_{2g}$ bands).
